# Supplementary material for: A Spark Optimizer for Adaptive, Fine-Grained Parameter Tuning
Source: arXiv:2403.00995 source file (2024-07-19)
Supplement: Supplementary file 1 [file appendix-model-udf.tex]

\section{Additional Details for Modeling}

\subsection{Diverse Queries in Spark.}
In big data analytics, Spark runs queries mainly in three types, (i) {\it pure SQL}, (ii) {\it SQL with UDFs}, and (iii) {\it SQL with ML tasks}. 
For example, the big data benchmark TPCx-BB~\cite{TPCx-BB} involves 30 frequently performed analytical queries, including 14 pure SQLs, 11 SQLs with UDFs, and 5 SQLs with ML tasks.

\subsection{Pure SQL Embedding and Modeling}

\subsubsection{Preliminary of the Transformer}

The transformer technology is proposed in \cite{attention} and quickly becomes popular for solving sequential tasks. 
Given a sequence of input $d$-dim vectors $\{x_i\}$, $i = 1...n$, the original transformer works as follows.

\minip{Positional Encoding.} For each position $i$, a cosine or sinusoidal function \cite{attention} is generated for $x_i$, and we get $h_i = x_i + PE_i \in \mathbb{R}^d$.

\minip{Attention Mechanism.} Feed $\{ h_i \}$ into a multi-layer transformer.
Each layer of the transformer involves a Multi-Head Attention (MHA) layer, stacked by $H$ identical attention blocks, and a position-wise Feed-Forward Network (FFN). 

The output of the MHA layer is a $n \times d$ matrix, as the output concatenation over each of $H$ heads, each of whose output is a $n \times \frac{d}{H}$ matrix. Each row $i$ in the output matrix $o_i$ corresponds to the input at the position $i$, and can be represented as follows.
\begin{align}
	o_i^k &= \sum_{j\in \mathcal{S}}a^k_{i,j}V_j^k, \text{where  } a^k_{i,j} =  \sigma(\frac{Q^k_i \cdot K^k_j}{\sqrt{d / H}}), k = 1...H \label{eq:attention-linear}\\
	o_i   &= W_o \|_{k=1}^H o_i^k
\end{align}
where $Q^k_i=W_Q^k h_i, K_i^k=W_K^k h_i, V_i^k = W_V^k h_i \in \mathbb{R}^{\frac{d}{H}}$ denote the three projections ($W_Q^k, W_K^k, W_V^k \in \mathbb{R}^{d\times \frac{d}{H}}$) of $h_i$ in the head $k$, representing the query, key, and value of itself;
$\mathcal{S}$ denotes the set of other inputs in the sequence;
$\sigma$ is the softmax function by iterating $j$ and the input of $\sigma$ is divided by $\sqrt{d/H}$ to avoid the vanishing gradient problem;
$W_o$ is a $d \times d$ matrix to be learned; 
and $\|$ denotes concatenation.

%Each head $k$ of the attention mechanism learns how each input $h_i$ correlated to other inputs in a subspace $k$ as $a^k_{i,j}, \forall j \in \mathcal{S}$, and selectively focuses on the correlated part with the weighted sum of $a^k_{i,j}$ and $V_j^k$ as the output. 

Inside each head $k$, it learns how an input $h_i$ correlated to other inputs via $a_{i,j}^k, \forall j\in \mathcal{S}$, and selectively focuses on the correlated part by the weighted sum of $a_{i,j}^k$ and $V_j^k$ to generate the output.

The output of the FFN layer is a $n\times d$ matrix, and each row of the output row $i$ ($\hat{\hat{h}}_i \in \mathbb{R}^d$) is transformed from $o_i$ over the FFN layer.
The FFN layer is fully connected and position-wise with two consecutive $d\times d$ affine projections.
It is further preceded and succeeded by residual connection \cite{ResidualConnection} and layer-normalization (Norm) layers \cite{LayerNorm} to avoid gradient vanishing. 
\begin{align}
	\hat{h}_i &= Norm(o_i + h_i), \;\;\;\;
	\hat{\hat{h}}_i = Norm(\hat{h}_i + FFN(\hat{h}_i)) \label{eq:ffn}
\end{align}

It is worth mentioning that $\hat{\hat{h}}_i$ is the $h_i$ in the next transformer layer, and the transformer sums up all $\{h_i\}$ in the last layer as the embedding for $\{x_i\}$ to be used for downstream tasks.

\subsubsection{Graph Transformer Network Embedder}

Our work applies the Graph Transformer Network (GTN) as the embedder~\cite{gtn-aaai21} to capture the query characteristics to align with the topology structure of the physical query plan in the Spark SQL.
Given a (sub)query plan as a DAG of operators $G=(V, E)$, assume we have $n$ operators encoded as $\{v_i\}$ and a set of dependencies $E$ representing the dataflow.

\minip{Laplacian Positional Encoding (LPE).} We use the graph laplacian positional encoding~\cite{lapPE} to map each operator into the Euclidean space while maintaining the association property among operators. Consider mapping $G=(V, E)$ to $\Lambda = \{ \lambda_i \} \in \mathbb{R}^{n\times d_0}$ (for $i=1...n$), where $\lambda_i \in \mathbb{R}^{d_0}$ is in the $d_0$-dim space. Two operators $v_i$ and $v_j$ are associated if and only if $v_i$ points to $v_j$ or $v_j$ points to $v_i$, denoted as $A_{ij} = 1$; otherwise, $A_{ij}=0$.
To maintain the association property after the mapping, the LPE minimizes the Euclidean distance as:
$$
\sum_{i,j}\| \lambda_i - \lambda_j \|^2 A_{ij} = \text{tr}(\Lambda^TL\Lambda)
$$
where $L = D - A$ is the laplacian matrix as the subtraction between the degree matrix D and the association (adjacent) matrix A in $G$.

Standard methods show that the solution is provided by the matrix of eigenvectors ($\Lambda$) corresponding to the lowest eigenvalues ($\lambda^*$) of the generated eigenvalue problem $L\Lambda = \lambda^* D \Lambda $.
Denote the set of the solved positional encodings as $\Lambda = \{\lambda_i\}$, so we have $h_i = v_i + W_{\lambda}\lambda_i$ for each operator, where $W_{\lambda} \in \mathbb{R}^{d\times d_0}$.

\minip{Graph Attention Mechanism.} The original mechanism learns attention from all other inputs. However, in a physical query plan $G=(V, E)$, each operator only relies on its child nodes.
Let us denote $\mathcal{N}_i$ as the set of child nodes of $v_i$. The graph attention mechanism modifies the original mechanism by only modifying the Eq \eqref{eq:attention-linear} for each attention head $k$ as follows (for simplicity, we drop the superscript $k$ on the right-hand side).
\begin{align}
	o_i^k = \sum_{j\in \mathcal{N}_i}a_{i,j}V_j, \text{where } a_{i,j} =  \sigma(\frac{Q_i \cdot K_j}{\sqrt{d / H}}) \label{eq:attention-gtn}	
\end{align}

\minip{Example.} Figure~\ref{fig:model-gtn-example} shows a GTN example over a DAG of 5 operators with two layers and two heads per layer. 
We first generate $\{v_1...v_5\} \in \mathbb{R}^d$ by operator encoding. With LPE, we get $\{ h_1...h_5 \}$ ($h_i = v_i + \lambda_i$) as the inputs to the first layer. 
Now we illustrate how to pass $h_i$ from the current layer to the next layer by taking $h_2$ as an example. 
Since $v_0, v_1$ are the two child nodes of $v_2$, we have $\mathcal{N}_i = \{0, 1\}$. 
Given each of the head $k \in \{1,2\}$, we calculate the output by following Eq \eqref{eq:attention-gtn}: $o_2^k = \sum_{j\in \{0,1 \}}a_{2,j} V_j \in \mathbb{R}^{\frac{d}{2}}$, where 
$a_{2,j} = \sigma(\frac{Q_2 \cdot K_j}{\sqrt{d/2}}) = \exp(\frac{Q_2 \cdot K_j}{\sqrt{d/2}})/(\exp(\frac{Q_2 \cdot K_0}{\sqrt{d/2}}) + \exp(\frac{Q_2 \cdot K_1}{\sqrt{d/2}})), \forall j \in \{ 0,1 \}$ with a  separate set of $\{a, Q, K, V \}$. 
We then get $o_2 \in \mathbb{R}^d$ as the concatenation of $o_2^0$ and $o_2^1$ and pass it over eq~\eqref{eq:ffn} to get the $h_2$ in the second layer.
In the last layer, we sum up the output $\{ h_i\}$ to get the query embedding for $G$: $E = \sum_i h_i$.

%$$ % for slides
%\sum_{j\in \{0,1\}} \sigma(\frac{Q_2\cdot K_j}{\sqrt{d/2}})V_j
%$$

\subsubsection{Comparison to SOTAs} 

\begin{table}[t]
\ra{1} 
\small
\newrobustcmd{\B}{\bfseries}
\caption{Comparison to SOTA Transformers for Queries}
\label{tab:trasformer-comparison}
\centering
	\begin{tabular}{l|c|c|c}\toprule
\B Property & RAAL & QueryFormer & Ours \\ \midrule
\B Positional Encoding & 1D & 1D & Graph \\ \midrule
\B Multi-head Attention & NO & YES & YES \\ \midrule
\B \begin{tabular}{@{}l@{}}Attention Focus On \\Child Nodes Only  \end{tabular}& YES & NO & YES\\ \midrule
\B \begin{tabular}{@{}l@{}}Attention Score Calculated \\ over the focused nodes \end{tabular} & NO & YES & YES\\
\bottomrule
	\end{tabular}
\end{table}

We listed our comparison with two state-of-the-art transformer-based modeling methods RAAL~\cite{RAAL} and QueryFormer~\cite{queryformer} for big data analytics systems in Table~\ref{tab:trasformer-comparison}. 

\minip{Positional encoding.} RAAL and QueryFormer map the position in the query plan tree to a linear position and apply the sequential PE accordingly. 

RAAL serializes a DAG of operators into a sequence according to the execution order (the reverse order of DFS). However, operators can run at the same time when resources are enough. E.g., two scan operators running in two separate stages can fetch data from the storage layer simultaneously. Therefore, RAAL oversimplifies the topology of the query plan. 
QueryFormer projects the position of each operator to its height in the query plan tree and hence cannot fully capture the graph structures neither.

Our method, instead, applies the Laplacian PE, which takes the graph topology as the input and maps the position of each operator into a fix-sized vector without losing the relative associations among operators~\cite{lapPE}.
	
\minip{Attention Mechanism.} RAAL and QueryFormer over-complex the attention mechanism by attending to additional operators other than the child ones for each operator, which involves much noisy information for learning, and hence is hard to scale up for more complex query plans. 
RAAL calculates the attention score of each operator by using all the operators, including additional noisy information from its ancestors.
QueryFormer pays attention to all the descendent operators for each operator. 

Instead, GTN only pays attention to the child operators, which naturally aligns with the data flow (dependency) and provides a good inductive bias~\cite{inductive-bias}. It is also computation-friendly to query plans with a large number of operators.
Moreover, GTN applies the multi-head attention mechanism, with each head mapping the DAG of inputs to a separate subspace, which has been verified~\cite{bert,xlnet} to perform better than the single-head attention used in RAAL.

\cut{
\subsection{SQL with UDFs/ML Tasks}

\subsubsection{Challenges}

\subsubsection{Auto-encoder Embedder~\chenghao{[Innovation 3]}} 

\subsection{Model Building}

Our model is composed of a workload embedder and a neural network regressor, as shown in Figure~\ref{fig:model-gtn-example} and \ref{fig:model-nnr}, respectively.
The workload embedding $E$ should satisfy three properties. 
\begin{enumerate}
	\item {\it Independence.} A workload embedding should be independent of other factors such as input meta information $M$, the system states $S$, and configurations $\bs{\theta}$.
	\item {\it Invariance.} A workload embedding should be invariant given the same workload.
	\item {\it Similarity Preserving.} Two workloads generated from the same templates should always have a closer distance than two workloads generated from different templates.
\end{enumerate}

%Let us denote $T$ as a template and $\tau$ to denote the template mapping function.
We use $i$ to indicate a workload, and hence $Q_i$ is the $i$-th workload and $I_i, M_i, \bs{\theta}_i$ are configuration, input meta information and machine system states corresponding to $Q_i$.

\minip{A pure SQL.} 
A cost-based optimizer (CBO) can analyze a pure SQL and exposes features for each node in the physical query plan. Therefore, we embed the workload directly from the physical query plan to keep it {\it independent} and {\it invariant}. 
Specifically, our embedder takes the node features as inputs and uses the graph transformer network (GTN)~\cite{gtn-aaai21} to further capture the inter-node correlation. 
\todo{add formulas and explanations to show how we capture the inter-node correlation and the loss function}
\todo{how to emphasize the similarity preserving?}

\minip{A SQL with UDF.}
Spark supports integrations of user-defined functions (UDF) of different types, such as scalar user-defined functions (sUDF), user-defined aggregation functions (UDAF), and user-defined tabular functions (UDTF). 
A user can program arbitrary functions in a UDF, and hence the CBO cannot fully understand a SQL with UDF.
Therefore, we apply a gray-box approach and use an auto-encoder (AE) to extract the embedding of a SQL with UDF. 

Our AE takes the runtime metrics of executors as the input $x$, and learns the bottleneck hidden layer $z$ to reconstruct itself as $\hat{x}$. 
We consider the bottleneck layer $z=[z^0, z^1, z^2, z^3]$ as the concatenation of workload embedding, input data information, machine system states, and configuration. 
Specifically, $z^0$ should cover both the information learned from CBO and its UDF, and we force the first $d$ dimensions in $z^0$ to match GTN's output and let the remaining dimensions in $z^0$ to learn the UDF automatically.

To achieve the goal, our loss function first includes five point-wise losses for the independence property of the workload 
\begin{align}
	loss_1 &= \sum_{i=1}^B ||x_i - \hat{x_i}||_2^2 \\
	loss_2 &= \sum_{i=1}^B ||z_i^1 - I_i||_2^2 & 
	loss_3 &= \sum_{i=1}^B ||z_i^2 - M_i||_2^2 \\ 
	loss_4 &= \sum_{i=1}^B ||z_i^3 - \bs{\theta}_i||_2^2 &
	loss_5 &= \sum_{i=1}^B ||z_i^0[0:d] - GTN(Q_i)||_2^2
\end{align}
where $B$ indicates the number of workloads in a batch.

To preserve the similarity of workloads in the same template, we construct $N$ triples $(z_i^{0}, z_i^{0+}, z_i^{0-})$ from the $B$ workloads, where $z_i^{0}$ is an anchor workload, and $z_i^{0+}$ is a workload from the same template as $z_i^{0}$, and $z_i^{0-}$ is from a different template. 
We then construct the triplet-loss~\cite{tripletloss} as follows,
\begin{align}
	loss_6 &= \sum_{i=1}^N \left [ || z_i^0 - z_i^{0+} ||_2^2 - || z_i^0 - z_i^{0-}||_2^2 + \alpha \right]_+, \\
	& \forall(z_i^0, z_i^{0+}, z_i^{0-}) \in \mathcal{T}
\end{align}
where $\alpha$ is a margin (constant) that is enforced between the positive and negative pairs. $\mathcal{T}$ is the set of all possible triplets in the batch, and $|\mathcal{T}| = N$. With the triplet-loss, the workload embedding is learned to always have a closer distance to the ones from the same template than those generated from a different template.

Therefore, we learn AE embedder via the loss
\begin{align}
	loss &= \sum_{i=1}^{6} w_i\cdot loss_i 
\end{align}
where $\forall w_i > 0$ and $\sum w_i = 1$. After learning the AE embedder towards the $loss$, we get $E=z^0$.

\minip{A pipeline of SQL and ML tasks.}
}

\cut{
\subsection{Hierarchical Modeling for a Pure SQL}

\todo{explain why to hierarchical modeling? Avoid the effects of stage pending and support stage-level optimization.}

\subsubsection{Modeling granularities}

We consider our modeling targets in the following granularities.

\begin{enumerate}
	\item Query-level. We use $l$ and $c$ to represent the end-to-end latency and total cost of query $Q$.
	\item Stage-level. We use $l_{s_i}$, and $c_{s_i}$ to represent the end-to-end latency and the total cost for stage $s_i$. Hence, the stage-level latency becomes
		$l_{s_i} = f(E_i, I_i, M_i, \bs{\theta})$, where $E_i$, $I_i$ and $M_i$ are the embedding of the subquery plan, the input meta, and cluster system state corresponding to the stage $s_i$ respectively.
	\item Task-level. We use $t_{s_i}$ to represent the summation of the latencies from all tasks in $s_i$. $t_{s_i} = h(E_i, I_i, M_i, \bs{\theta})$
\end{enumerate}

\subsubsection{Compose the SQL latency from stages}

\todo{for FIFO and FAIR}
}

\subsection{SQL with UDF}
\label{appendix:model-udf}

Spark supports integrations of user-defined functions (UDF) of different types, such as scalar user-defined functions (sUDF), user-defined aggregation functions (UDAF), and user-defined tabular functions (UDTF). 
A user can program arbitrary functions in a UDF, and hence the CBO cannot fully understand a SQL with UDF.
Therefore, we apply a gray-box approach and use an auto-encoder (AE) to extract the embedding of a SQL with UDF. 

Our AE takes the runtime metrics of executors as the input $x$, and learns the bottleneck hidden layer $z$ to reconstruct itself as $\hat{x}$. 
We consider the bottleneck layer $z=[z^0, z^1, z^2, z^3]$ as the concatenation of workload embedding, input data information, machine system states, and configuration. 
Specifically, $z^0$ should cover both the information learned from CBO and its UDF, and we force the first $d$ dimensions in $z^0$ to match GTN's output and let the remaining dimensions in $z^0$ to learn the UDF automatically.

To achieve the goal, our loss function first includes five point-wise losses for the independence property of the workload 
\begin{align}
	loss_1 &= \sum_{i=1}^B ||x_i - \hat{x_i}||_2^2 \\
	loss_2 &= \sum_{i=1}^B ||z_i^1 - I_i||_2^2 & 
	loss_3 &= \sum_{i=1}^B ||z_i^2 - M_i||_2^2 \\ 
	loss_4 &= \sum_{i=1}^B ||z_i^3 - \bs{\theta}_i||_2^2 &
	loss_5 &= \sum_{i=1}^B ||z_i^0[0:d] - GTN(Q_i)||_2^2
\end{align}
where $B$ indicates the number of workloads in a batch.

To preserve the similarity of workloads in the same template, we construct $N$ triples $(z_i^{0}, z_i^{0+}, z_i^{0-})$ from the $B$ workloads, where $z_i^{0}$ is an anchor workload, and $z_i^{0+}$ is a workload from the same template as $z_i^{0}$, and $z_i^{0-}$ is from a different template. 
We then construct the triplet-loss~\cite{tripletloss} as follows,
\begin{align}
	loss_6 &= \sum_{i=1}^N \left [ || z_i^0 - z_i^{0+} ||_2^2 - || z_i^0 - z_i^{0-}||_2^2 + \alpha \right]_+, \\
	& \forall(z_i^0, z_i^{0+}, z_i^{0-}) \in \mathcal{T}
\end{align}
where $\alpha$ is a margin (constant) that is enforced between the positive and negative pairs. $\mathcal{T}$ is the set of all possible triplets in the batch, and $|\mathcal{T}| = N$. With the triplet-loss, the workload embedding is learned to always have a closer distance to the ones from the same template than those generated from a different template.

Therefore, we learn AE embedder via the loss
\begin{align}
	loss &= \sum_{i=1}^{6} w_i\cdot loss_i 
\end{align}
where $\forall w_i > 0$ and $\sum w_i = 1$. After learning the AE embedder towards the $loss$, we get $E=z^0$.

%\minip{A pipeline of SQL and ML tasks.}

\minip{Justify why it is a good design.} The goal of the AE is to get the encoding $z$ which involves the independent factors affecting the runtime metrics $x$, so we consider learning $z$ as stacking of
\begin{enumerate}
	\item Workload embedding $z^0$
	\item Input data information $z^1$
	\item Machine system states $z^2$
	\item Spark configuration $z^3$
\end{enumerate}
Regarding SQL with UDF, we use our trained GTN embedder (designed for SQL workloads) to embed the SQL structure (a DAG of query operators, with each node encoded by operator type and cardinality estimations). We use the $z^0[0:d]$ to learn this SQL-related embedding, while the $z^0[d:]$ is utilized to learn unrepresented information related to UDF in the target query.

\subsection{Model Clarifications}

\minip{How to choose the readout function (from \texttt{mean}, \texttt{sum}, \texttt{max}) in a Graph-based model?}  
% When we have UDF in stage 1 and SQL in stage 2, what aggregate operator makes sense to combine their encodings?  Sum or max, or average?

Technically, all the readout functions make sense because they can all contribute to the forward path in a NN model. We usually do hyperparameter tuning to decide which one to choose based on the performance. However, there are some common rules to compare among them generally:
\begin{enumerate}
	\item We prefer sum/mean to max because sum and mean could force more neurons and weights to participate in learning during each backpropagation path.
	\item Whether to choose sum or mean also depends on which graph neural network (GNN) work structure we target. GNN has different variants, some suit sum (such as GIN) and some suit mean (such as GCN).
	\item When doing hyperparameter tuning for Graph Transformer Network (GTN), I also observed mean $\approx$ sum < max in WMAPE.
\end{enumerate}
