# Supplementary material for: A Spark Optimizer for Adaptive, Fine-Grained Parameter Tuning
Source: arXiv:2403.00995 source file (2024-07-19)
Supplement: Supplementary file 2 [file appendix-spark.tex]

\section{Additional Details in Spark}

\subsection{Optimization Rules}
\label{appendix:optimization-rules}
Figure~\ref{fig:opt-rules} illustrates the transformations of a collapsed LQP and a runtime QS, which both pass through a pipeline of parametric rules (blue) and non-parametric rules (gray). \todo{revise the diagram.}
\begin{figure}[t]
	\centering
	\captionsetup{justification=centering}
	\includegraphics[width=.5\linewidth,height=3cm]{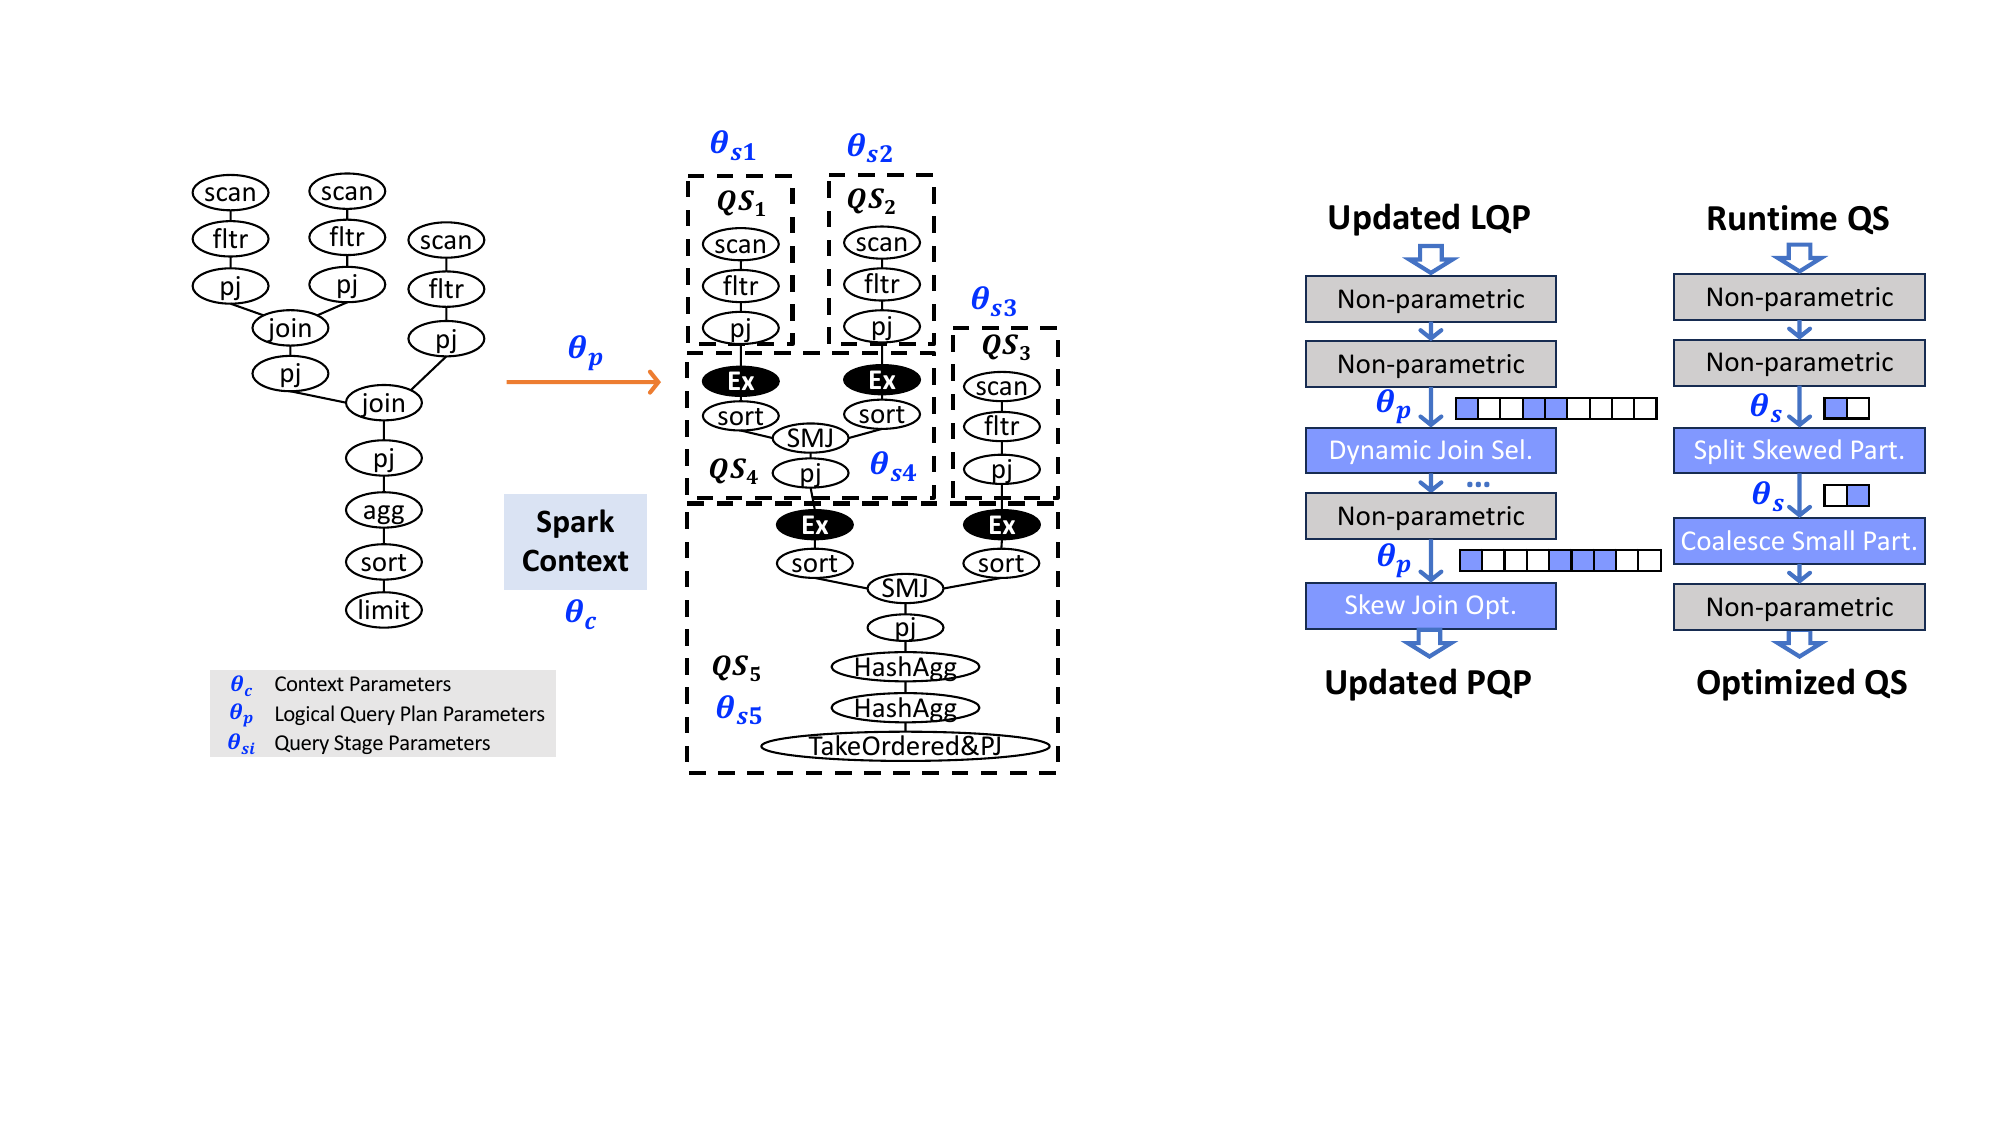}
	\captionof{figure}{\small{Runtime Opt. Rules}}
	\label{fig:opt-rules}
\end{figure}

\subsubsection{Query Optimization Rules.}
\label{appendix:lpq-rules}

\subsubsection{Query Stage Optimization Rules.}
\label{appendix:qs-rules}

\subsection{Mixed Decision Space}
\label{appendix:mixed-decision-space}

\begin{figure}
\centering
\captionsetup{justification=centering}
  \centering
  \includegraphics[height=6cm,width=8cm]{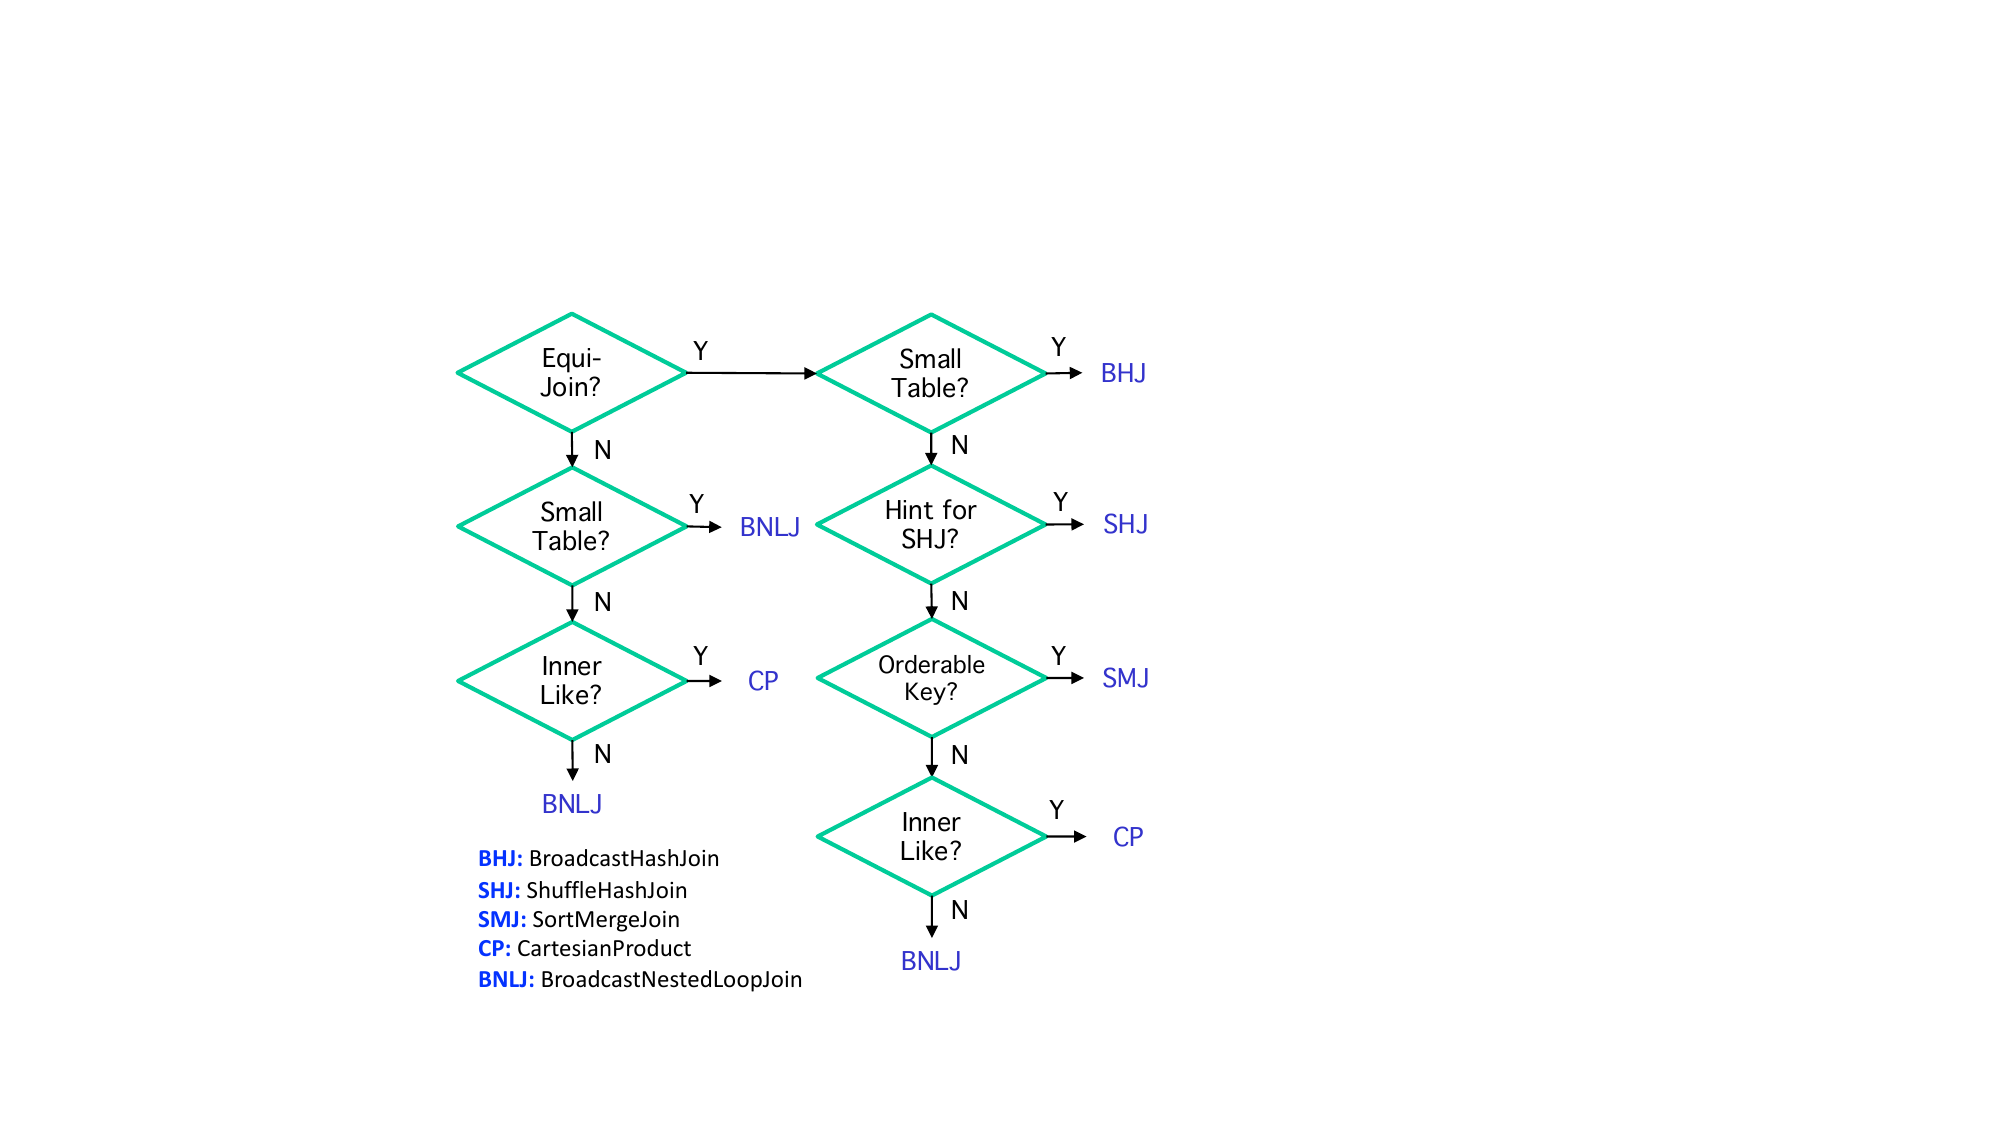}
  \captionof{figure}{\small{Join Selection Strategy}}
  \label{fig:join-sel}
\end{figure}

The configuration parameters $\thetabm$ introduce a mixed decision space for optimization when the adaptive query execution is enabled (as by default).
Runtime parameters ($s_1$ - $s_4$) are plan-dependent and can alter the physical plan given a fixed optimized logical plan. 
For instance, ($s_1$ - $s_4)$ will jointly be used to derive the internal join hint and further decide the physical operator join type in AQE.
Other parameters in our selected list are plan-independent and do not impact the physical plan. They are either the general Spark parameters ($k_1$ - $k_8$) or SQL parameters that only affect the parallelism ($s_5$ - $s_9$). 
Therefore, tuning Spark parameters requires making decisions in both the physical plan space and numerical space for the plan-independent parameters, which is more challenging compared to the approaches that focus solely on plan-independent parameters~\cite{cleo-sigmod20,adaptive-code-learning-spark-icde22,LyuFSSD22,LOCAT-sigmod22}.

\minip{Join Selection Logistics.} During query execution, the query optimizer performs a two-step re-optimization process to determine the physical join type based on runtime statistics.

In the first step, the AQEOptimizer applies the \textit{DynamicJoinSelection} rule to the logical plan, generating an internal join hint. 
This rule aims to avoid a broadcast join when the ratio of empty partitions exceeds the threshold ($s_2$), and to prioritize a shuffle-hash join when both the advisory partition size ($s_1$) and the size of each partition are below a separate threshold ($s_3$).

In the second step, the query optimizer selects the join type based on a decision tree, as shown in Figure~\ref{fig:join-sel}. 
For equi-joins, it attempts to use a \textit{BroadcastHashJoin (BHJ)} when any table's size is smaller than the threshold ($s_4$). When the condition is not met, it selects \textit{ShuffleHashJoin (SHJ)} when a shuffle-hash preference exists from the first step. If the join key is orderable, it opts for a \textit{SortMergeJoin (SMJ)}. If none of these conditions apply, it resorts to a \textit{CartesianProduct (CP)} for inner joins and selects \textit{BroadcastNestedLoopJoin (BNLJ)} as the final option. For non-equi-joins, it chooses either \textit{BNLJ} or \textit{CP} based on the input size and whether it is an inner join.

During the evaluation using the TPCH benchmark, Spark covers {\it BHJ, SHJ, SMJ} for equi-joins, and {\it BNLJ} for non-equi-joins.

\subsection{Simplification for the Mixed Decision Space.} 
\label{appendix:mixed-decision-space-simplification}

We demonstrate the simplification of the mixed decision space by tuning all parameters based on the optimized logical plan to bypass the choice of the physical plan. 

\minip{Workload.} Our workload consists of 22 default TPCH queries. For each query, we generate 180 combinations by varying the plan-dependent parameters $s_1$ - $s_4$ while keeping other parameters fixed. We run each unique pair (query, configuration) 3 times and pick the median latency as the target objective.

\minip{Models.} We compare the performance of two types of models.
(1) The \texttt{PP-agnostic} model is trained using physical-plan-agnostic features, including the optimized logistic plan, and plan-dependent parameters.
(2) The \texttt{PP-aware} model is trained using physical-plan-aware features, including the optimized logistic plan, physical plan, and plan-dependent parameters.
%Both models have access to the plan-dependent parameters ($s_1$ - $s_4$) and the optimized logical plan.

\begin{figure}
  \centering
  \begin{tabular}{l}
		\subfigure[\small{Compare over Weighted Mean Absolute Percentage Error (WMAPE)}]
		{\label{fig:model-agnostic-wmape}\includegraphics[width=.98\linewidth]{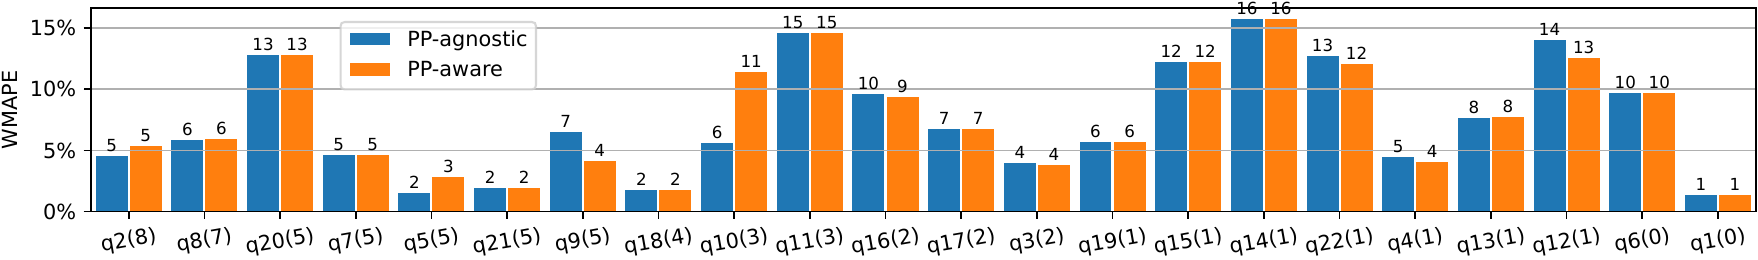}}
		\\
		\subfigure[\small{Compare over Mean Absolute Percentage Error (MAPE)}]
		{\label{fig:model-agnostic-mape}\includegraphics[width=.98\linewidth]{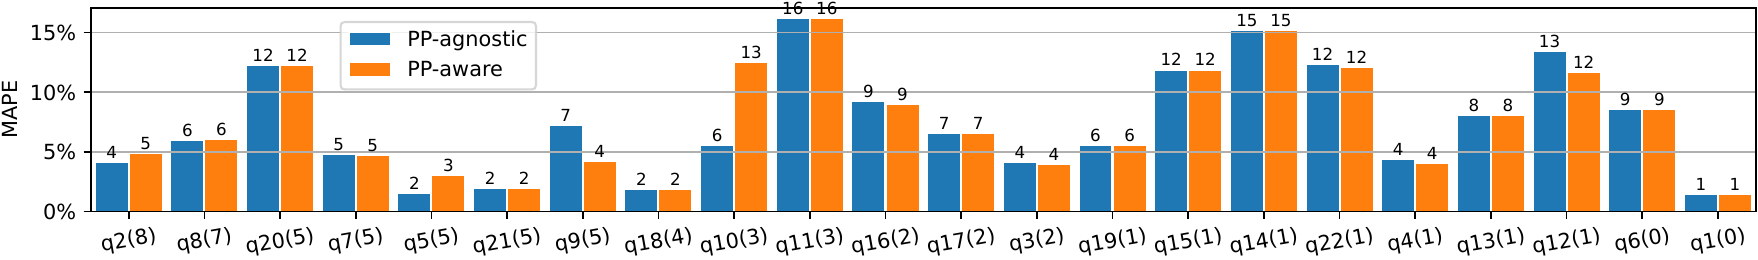}}
		\\
		\subfigure[\small{Compare over Median Percentage Error (MdErr)}]
		{\label{fig:model-agnostic-mderr}\includegraphics[width=.98\linewidth]{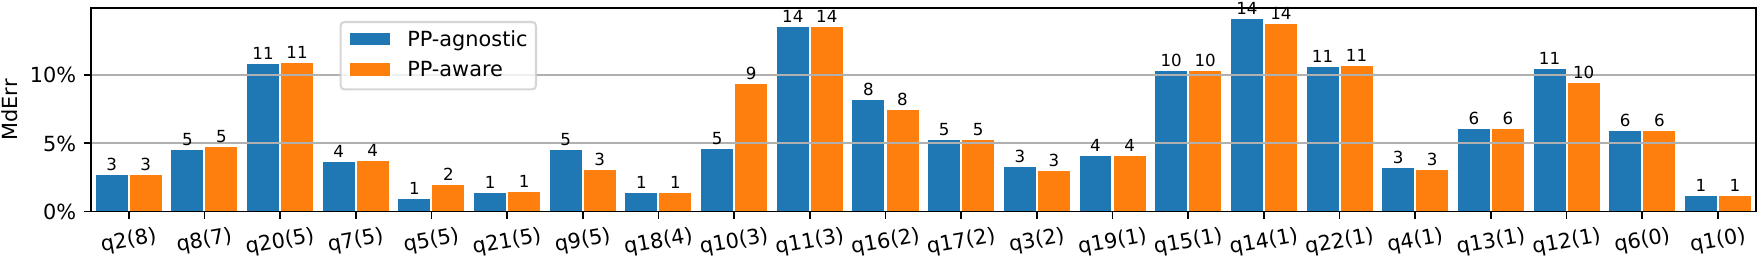}}
		\\
		\subfigure[\small{Compare over 90\%tile Percentage Error (90\%Err)}]
		{\label{fig:model-agnostic-90err}\includegraphics[width=.98\linewidth]{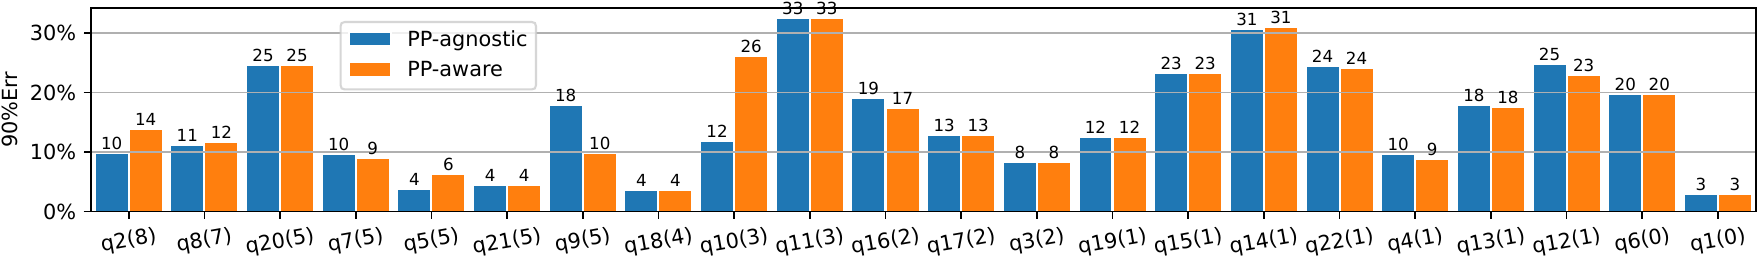}}
		\\
		\subfigure[\small{Compare over 99\%tile Percentage Error (99\%Err)}]
		{\label{fig:model-agnostic-99err}\includegraphics[width=.98\linewidth]{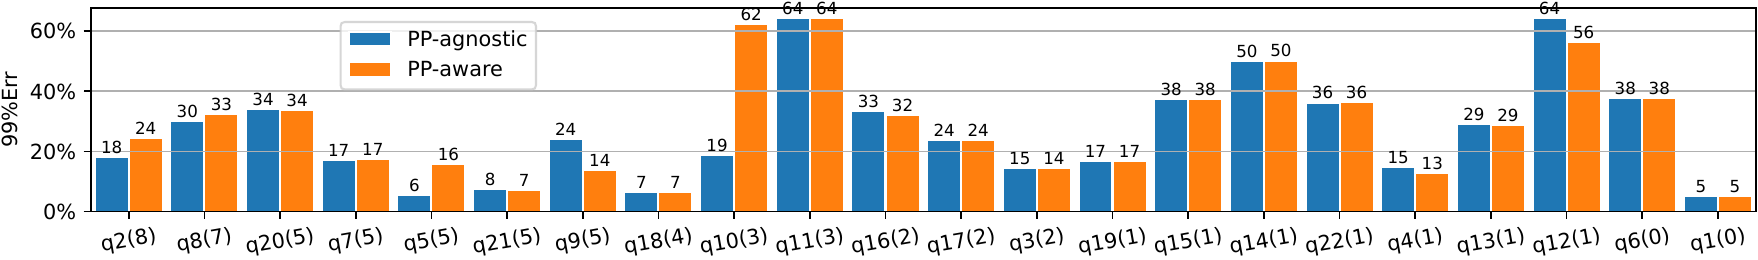}}						
  \end{tabular}
  \captionof{figure}{\small{Model performance comparison between physical plan agnostic features and physical plan aware features}}
  \label{fig:pp-ag-vs-aw}
\end{figure}

\minip{One-model-per-query.} We first train a separate model for each query. Each model is trained using 180 data points specific to that query. Consequently, these data points share common general Spark parameters, input data characteristics, and an optimized logical plan within the input feature space. As a result, we exclude the common features in both types of models to simplify the comparison.

During the evaluation, the \texttt{PP-agnostic} model utilizes $s_1$ - $s_4$ to predict the latency, while the \texttt{PP-aware} model incorporates $s_1$ - $s_4$ and a list of join types used in the physical plan for the latency prediction. 
We employ XGBoost as the predictive model and use the mean absolute error (MAE) as the loss function to align with our primary metric Weighted Mean Absolute Percentage Error (WMAPE). Each model undergoes training with ~150 hyperparameters and presents the metrics based on the average form a 5-fold cross-validation. 

Figure~\ref{fig:pp-ag-vs-aw} illustrates that the \texttt{PP-agnostic} model exhibits a closely aligned predictive performance with the \texttt{PP-aware} model across various significant metrics. 
This observation confirms the intuition that the physical plan and plan-dependent parameters possess a strong correlation, given an optimized logical plan.

Consequently, our focus lies in the parameter tuning based on the {\bf optimized logical plan} to address the mixed decision plan challenge and bypass the complexities associated with choosing physical plans.

%We show our comprehensive comparison in Figure~\ref{fig:pp-ag-vs-aw} over the five metrics: the weighted mean absolute percentage error (WMAPE), the mean absolute percentage error (MAPE), the median percentage error (MdErr), the 90\%-tile percentage error (90\%Err), and the 99\%-tile percentage error (99\%Err).

\minip{One-model-for-all.} \todo{when have more time}
