# Supplementary material for: A Spark Optimizer for Adaptive, Fine-Grained Parameter Tuning
Source: arXiv:2403.00995 source file (2024-07-19)
Supplement: Supplementary file 3 [file appendix-trace-collection.tex]

\section{Additional Details In Trace Collection}

\subsection{Query stage to stage mapping}

During AQE, each query stage (QS) is submitted as a Spark job for execution. 
Therefore, the QS metrics should be aggregated from the metrics of the corresponding Spark stages in the submitted job.

To build the mapping, we did the following steps.
\begin{itemize}
	\item We group the Spark stages into "Stage Groups (SG)" by the RDD scope IDs and record the SG execution order. 
	\item We set a table keyword for each SG. For the scan-based SGs, we use the name of the table being scanned; for the follow-up SGs, we use an empty string "".
	\item At the QS submission, we injected a customized listener {\it onQueryStageSubmitted} to capture (1) the QS submission order, (2) the query ID, (3) the query IDs of the corresponding subqueries, (4) whether the QS belongs to a subquery, and (5) the corresponding table keyword.
	\item When the SQL is completed, we replay the execution order of QSs based on their submission order and subquery dependencies.
	\item We match the QS and SG based on their execution order in their corresponding table keyword.
\end{itemize}

It is worth mentioning that
\begin{itemize}
	\item Spark stages from the same QS will have duplicated RDD executions (e.g., when doing sort operation), reflecting the identical RDD scope Ids. We group those stages into one SG to map to a QS.
	\item Parallel scan-based QSs are submitted for execution asynchronously. So, their submission order does not always match the execution order. To address the issue, we further use the table keyword to distinguish the parallel scan-based QSs.
\end{itemize}
